# Supplementary material for: Towards Responsible Governance of Biological Design Tools
Source: arXiv:2311.15936 ancillary file (2023-11-30)
Supplement: Supplementary file 1 [file Supplementary_Material.pdf]

## Supplementary Table 1: Governance measures' feasibility and compatibility with open-source

We consider a model 'open-source' (OS), if model weights and accompanying code has been freely published on the internet, typically under an open-source license.

| Measure | Technically compatible? | Feasible to implement? |
|---|---|---|
| Responsible Development | | |
| 1. Expanded Dual-Use Review | ✔ | ✔ |
| 2. Model Licensing for Training or Release | ✔ | OS may be exempt |
| 3. Expanded Developer Liability | ✔ | OS may be exempt |
| 4. Voluntary Commitments | ✔ | ✔ |
| 5. Export Controls | ✔ | OS may be exempt |
| 6. Publication Norms | ✔ | ✔ |
| Risk Assessment | | |
| **7. Model Evaluations** | ✔ | ✔ |
| 8. Red Teaming | ✔ | ✔ |
| 9. Monitoring for Misuse | ❌ (needs structured access) | More difficult |
| Transparency | | |
| 10. Impact Statements | ✔ | ✔ |
| 11. Information-Sharing with Regulators | ✔ | ✔ |
| **12. Vulnerability Reporting** | ✔ | ✔ |
| 13. Watermarking | ❌ (may be fine-tuned away) | More difficult |
| Access Management | | |
| 14. Data Curation | ✔ | ✔ |
| 15. Data Use Agreements | ✔ | ✔ |
| **16. Structured Access** | ❌ | More difficult |

| | | |
|---|---|---|
| **17. Know Your Customer** | ❌ (needs structured access) | More difficult |
| **18. NA Synthesis Screening** | ✔ | ✔ (external to models) |
| 19. Input/Output Filtering | ❌ (may be fine-tuned away) | ✔ |
| Cybersecurity | | |
| 20. Database Security | ✔ | ✔ |
| 21. Securing Weights | ❌ | ❌ |
| **22. Securing Lab Equipment** | ✔ | ✔ (external to models) |
| Investing in Resilience | | |
| 23. Public Compute | ✔ | ✔ |
| **24. Model-Sharing Infrastructure** | ✔ | ✔ |
| 25. Fund Countermeasures | ✔ | ✔ |
